# Supplementary material for: Agents Thinking Fast and Slow: A Talker-Reasoner Architecture
Source: arXiv:2410.08328 source file (2024-10-10)
Supplement: Supplementary file 1 [file appendix.tex]

%\subsubsection{Updating Belief State based on new world observations}

\begin{quote}
\small{
    \fon{cmr}{
    \textbf{BELIEF in \texttt{mem}:}
    \{updated context: starting context, 
updated journey title: Sleeping Coaching, 
user context: UserCollectedContextData(
primary sleep concern: Eliminate distractions (noise and light),
user barriers: Noisy environment; Light distractions, 
recommendations: Use blackout curtains or blinds; Consider noise-cancelling curtains or soundproofing panels; Avoid blue light; Dimmable lights; Use low-wattage night lights with warm soft colors, 
coaching phase: CoachingPhase(PLANNING)\}
    }
    }
\end{quote} 
\section{Example of a conversation}
\begin{quote}
    \fon{cmr}{Hey what's up?} 
\end{quote}

\begin{figure}[!h]
\begin{minipage}[b]{0.5\linewidth}
\begin{beliefstate}
updated context: starting context \\
updated journey title: Sleeping Coaching \\
coaching phase: CoachingPhase:
value: UNDERSTANDING
\end{beliefstate}
\caption{Beginning belief state}
\end{minipage}
\begin{minipage}[b]{0.5\linewidth}
\begin{beliefstate}
updated context: starting context \\
updated journey title: Sleeping Coaching \\
user collected context data: UserCollectedContextData: 
primary sleep concern: Eliminate distractions (noise and light)\\
user barriers: 
\begin{itemize}
    \item Noisy environment
    \item Light distractions
\end{itemize}\\
recommendations:
\begin{itemize}
    \item Use blackout curtains or blinds
    \item Consider noise-cancelling curtains or soundproofing panels
    \item Avoid blue light
    \item Dimmable lights
    \item Use low-wattage night lights with warm soft colors
\end{itemize}\\
coaching phase: CoachingPhase:
value: PLANNING
\end{beliefstate}
\caption{Updated fields in belief state after user-AI Coaching Agent interactions \kc{see if we should provide this in XML / JSON format instead.}}
\end{minipage}
\end{figure}

\begin{user}
Thanks! Can you now help me set goals around eliminating anxious thoughts and creating my serene background?
\end{user}

%\begin{reasoner}
%woohoo
\begin{beliefstate}
user collected context data: UserCollectedContextData: primary sleep concern: anxious thoughts \\
...\\
coaching phase: CoachingPhase: value: GOAL SETTING
\end{beliefstate}
%\end{reasoner}

\begin{talker}
conversational response:
\end{talker}
